# Supplementary material for: Constrained Pure Exploration Multi-Armed Bandits with a Fixed Budget
Source: arXiv:2211.14768 source file (2022-11-27)
Supplement: Supplementary file 1 [file appendix_B.tex]

\section{Proof of Conjecture \ref{thm: K arms lb} for special cases} \label{app: K arms lb}
\subsection{All arms are infeasible}
We first prove Conjecture \ref{thm: K arms lb} for the case when all arms are infeasible. Here, the error event corresponds to the algorithm incorrectly identifying the instance as being feasible. Informally, we would expect this to depend upon the minimum infeasibility gap among all arms, which is what happens. This is similar to the Thresholding Bandit Problem (refer to \cite{tbp-locatelli16}) in the sense that one only has to identify whether each arm is above or below a given threshold, but is a different problem as this 

\begin{proof}
Consider any alternative bandit model $\nu^{\prime}$ with at least one feasible arm. Extending \eqref{eqn: kaufmann_lemma1} for $K$ arms on the the event $\mathcal{D}= \{ \hat{O}([K]) \neq 0 \}$, we get: 
\begin{align*}
\sum_{i=1}^{K}\mathbb{E}_{\nu^{\prime}}\left[N_{i}(T)\right] \textrm{KL}\left(\nu^{\prime}(i), \nu(i)\right) \geq d\left(\mathbb{P}_{\nu^{\prime}}(\mathcal{D}), \mathbb{P}_{\nu}(\mathcal{D})\right),
\end{align*}
where $\mathbb{E}_{\nu}(\cdot)$ and $\mathbb{P}_{\nu}(\cdot)$ denotes the expectation and the probability respectively with respect to the randomness introduced by the interaction of the algorithm with the bandit instance $\nu$, and $d(\cdot, \cdot)$ denotes the binary relative entropy. Denote by $e_T(\nu)$ the probability of error of the algorithm on the instance $\nu$.

We have that $e_{T}(\nu)=1-\mathbb{P}_{\nu}(\mathcal{D})$ and $e_{T}\left(\nu^{\prime}\right) \geq \mathbb{P}_{\nu^{\prime}}(\mathcal{D})$. As algorithm $\mathcal{L}$ is consistent, we have that for every $\epsilon>0, \exists T_{0}(\epsilon)$ such that for all $T \geq T_{0}(\epsilon), \mathbb{P}_{\nu^{\prime}}(\mathcal{D}) \leq \epsilon \leq \mathbb{P}_{\nu}(\mathcal{D})$. For
$T \geq T_{0}(\epsilon)$, we have:
\begin{align*}
\sum_{i=1}^{K}\mathbb{E}_{\nu^{\prime}}\left[N_{i}(T)\right] \textrm{KL}\left(\nu^{\prime}(i), \nu(i)\right)  &\geq d\left(\epsilon, 1-e_{T}(\nu)\right) \\& \geq(1-\epsilon) \log \frac{1-\epsilon}{p_{T}(\nu)}+\epsilon \log \epsilon. 
\end{align*}
In the limit where $\epsilon$ goes to zero, we have,
\begin{align*}
\limsup_{T \rightarrow \infty}-\frac{1}{T} \log e_{T}(\nu) &\leq \limsup_{T \rightarrow \infty} \sum_{j=1}^{K} \frac{\mathbb{E}_{\nu^{\prime}}\left[N_{j}(T)\right]}{T} \textrm{KL}\left(\nu^{\prime}(j), \nu(j)\right) \\
&\leq \max_{j \in [K]} \textrm{KL}\left(\nu^{\prime}(j), \nu(j)\right).
\end{align*}
Denote by $\mathcal{M}$ the set of two-armed bandit instances whose arms belong to $\mathcal{G}$. Minimizing the RHS over all feasible instances in $\mathcal{M}$ gives us:
\begin{align*}
\limsup_{T \rightarrow \infty}-\frac{1}{T} \log e_{T}(\nu) \leq \underset{\nu^{\prime} \in \mathcal{M}: O(\nu^{\prime} ) \neq 0 }{\inf} \max_{j \in [K]} \textrm{KL}\left(\nu^{\prime}(j), \nu(j)\right). \numberthis \label{eqn: kaufmann_K}
\end{align*}
Using the formula for the KL divergence between two multivariate distributions in \eqref{eqn: kaufmann_K} gives:
\begin{align*}
&\limsup_{T \rightarrow \infty}-\frac{1}{T} \log e_{T}(\nu) \\
&\leq \underset{\nu^{\prime} \in \mathcal{M}: O(\nu^{\prime} ) \in \{0,1,2\} \setminus \{O(\nu)\}}{\inf} \underset{i \in [K]}{\max} a_1\left(\mu_{1}(i)-\mu_{1}^{\prime}(i)\right)^2 \\
&+  a_2\left(\mu_{2}(i)-\mu_{2}^{\prime}(i)\right)^2 . \numberthis \label{eqn: gaps_lb_K} 
\end{align*}
The infimum is obtained in \eqref{eqn: gaps_lb_K} when $\nu^{\prime}$ is such that only arm 1 is feasible with $\mu_1(1)=\mu_1^{\prime}(1)$ and the other infeasible arms coincide with the corresponding infeasible arms of $\nu$ (i.e., both attributes are the same).Thus, we get
\begin{align*}
\limsup_{T \rightarrow \infty}-\frac{1}{T} \log e_{T}(\nu) \leq a_2 \left ( \mu_2(1)-\tau\right )^2
\end{align*}
 Note that when two arms are infeasible, we have $\Delta(i.j)=\sqrt{a_2} \min \left \{ \mu_2(i)-\tau, \mu_2(j)-\tau \right \}$. As arm 1 has the least infeasibility gap by definition, $H_1=\frac{K}{a_2\left ( \mu_2(1)-\tau\right )^2}$  and thus we get the form in Conjecture \ref{thm: K arms lb} with $d=K$. 
\end{proof}

\subsection{All arms are feasible}

When all arms are feasible, the error event corresponds to the algorithm incorrectly identifying the instance as being infeasible or recommending an arm other than the optimal arm.
