# Supplementary material for: Constrained Pure Exploration Multi-Armed Bandits with a Fixed Budget
Source: arXiv:2211.14768 source file (2022-11-27)
Supplement: Supplementary file 2 [file appendix_E.tex]

\section{Some more numerical experiments} \label{app: num_exps}
